# Supplementary material for: Direct Retrieval-augmented Optimization: Synergizing Knowledge Selection and Language Models
Source: arXiv:2505.03075 source file (2025-05-05)
Supplement: Supplementary file 1 [file 08-appendix.tex]

% 
